# Supplementary material for: Model CBOR Serialization for Federated Learning
Source: arXiv:2401.14056 source file (2024-01-25)
Supplement: Supplementary file 1 [file 99-appendix.tex]

\section*{Appendix}

\begin{listing}[!ht]
\inputminted[]{cddl}{cddl/full.txt}
\caption{Full CDDL description of the messages}
\label{lst:cddl}
\end{listing}

\begin{listing}[!ht]
\inputminted[]{protobuf}{protobuf/full.txt}
\caption{Full Protobuf description of messages}
\label{lst:pb}
\end{listing}
